# Supplementary material for: Visibly Linear Dynamic Logic
Source: arXiv:1512.05177 source file (2017-05-17)
Supplement: Supplementary file 1 [file appendix.tex]

\section{Appendix}
